# Supplementary material for: Attention-based Audio-Visual Fusion for Robust Automatic Speech Recognition
Source: arXiv:1809.01728 source file (2019-05-01)
Supplement: Supplementary file 1 [file s_appendix.tex]

% \documentclass[sigconf]{acmart}

% \begin{document}

\appendix
\section{Numerical Results}

\begin{table}[h]
\centering
\footnotesize
\caption{Character Error Rate (CER) / Word Error Rate (WER)  [\%] on TCD-TIMIT}
\label{res:tcd}
\begin{tabular}{lllll}
% \hline

                      & \textbf{clean} & \textbf{10db} & \textbf{0db} & \textbf{-5db} \\ \hline

\textbf{A - WGN} & 19.16 / 45.53 & 25.58 / 53.89 & 34.92 / 64.98 & \\ %\hline
\textbf{A - Cafe} & 19.16 / 45.53 &  25.61 / 54.48 & 38.39 / 68.70 & 46.52 / 76.44 \\ %\hline
\textbf{A - Street} & 19.16 / 45.53 &  24.44 / 52.46 & 34.56 / 64.81 & 41.58 / 71.06 \\ %\hline

\hline

\textbf{AV Cat - WGN}   & 20.69 / 51.88 & 29.02 / 63.77 & 39.81 / 75.55 &  \\ %\hline
\textbf{AV Cat - Cafe} & 20.69 / 51.88 & 29.19 / 63.12 & 43.69 / 79/26 & 51.95 / 86.78  \\ %\hline
\textbf{AV Cat - Street} & 20.69 / 51.88 & 26.87 / 60.61 & 38.95 / 74.31 & 47.00 / 81.06  \\ %\hline

\hline

\textbf{AV Align - WGN}   & \textbf{17.70} / 41.90 & \textbf{23.65} / 49.95 & \textbf{29.68} / 57.07 &  \\ %\hline
\textbf{AV Align - Cafe}   & \textbf{17.70} / 41.90 & \textbf{24.23} / 51.94 & \textbf{31.93} / 60.88 & \textbf{32.68} / 60.58 \\ %\hline
\textbf{AV Align - Street}   & \textbf{17.70} / 41.90 & \textbf{22.66} / 49.73 & \textbf{27.92} / 55.19 & \textbf{28.72} / 55.63 \\ %\hline

\end{tabular}
\end{table}

\begin{table}[h]
\centering
\footnotesize
\caption{Character Error Rate (CER) / Word Error Rate (WER)  [\%] on LRS2}
\label{res:mvlrs}
\begin{tabular}{lllll}
%\hline
                      & \textbf{clean} & \textbf{10db} & \textbf{0db} & \textbf{-5db} \\ \hline
                      
\textbf{A - WGN} &  14.29  /  29.90          &    20.45 / 39.17        &    34.95   / 57.90      & \\ %\hline
\textbf{A - Cafe} & 14.29  /  29.95 &  \textbf{18.72} / 36.73 & \textbf{30.93} / 53.10  & 41.88 / 66.64 \\ %\hline
\textbf{A - Street } & 14.29  /  29.95 & \textbf{17.11} / 34.12 & \textbf{28.62} / 50.19 & 38.51 / 62.25 \\ %\hline

\hline

\textbf{AV Cat - WGN}   &     17.40  / 37.43         &     24.52 / 47.61         &  40.96  / 68.64    &   \\ %\hline

\hline

\textbf{AV Align - WGN}   &  \textbf{14.11} / 30.48 & \textbf{19.96} / 39.68 &  \textbf{33.94} / 57.89  &\\ %\hline
\textbf{AV Align - Cafe}   & \textbf{14.11} / 30.48 & 18.93 / 38.11 &  31.65 / 54.35  & \textbf{41.47} / 66.10 \\ %\hline
\textbf{AV Align - Street}   & \textbf{14.11} / 30.48 & 18.18 / 36.47 &  29.26 / 51.29  & \textbf{37.97} / 61.83\\ %\hline
\end{tabular}
\end{table}

% \end{document}
